# Supplementary material for: From General to Specific: Informative Scene Graph Generation via Balance Adjustment
Source: arXiv:2108.13129 source file (2021-08-30)
Supplement: Supplementary file 1 [file 04142-supp.pdf]

# Supplementary Material for "From General to Specific: Informative Scene Graph Generation via Balance Adjustment"

Yuyu Guo[1] Lianli Gao[1*] Xuanhan Wang[1] Yuxuan Hu[2] Xing Xu[1] Xu Lu[3]
Heng Tao Shen[1] Jingkuan Song[1]

[1]Center for Future Media & School of Computer Science and Engineering,
University of Electronic Science and Technology of China, China

[2]Southwest University, China [3]Kuaishou, China

## Abstract

*Due to the page limitation of the paper, we further illustrate our method in this supplementary material, which contains the following sections: 1). Review of the baseline models; 2). Supplementary quantitative results; 3). Supplementary visualization results; and 4). Conclusion.*

## 1. Review of Baseline Models

In our experiments, we used three baseline models, *i.e.*, **MotifNet**, **VCTree** and **Transformer**, to verify our method. These models are reviewed as follows:

**MotifNet**: Zellers *et al.* [7] explored regularly appearing substructures, namely motifs, in scene graphs. In order to capture the high-level motifs, they introduced MotifNet to encode the global context. Besides MotifNet, a strong baseline based on the dependency between instance labels and predicate categories was proposed to enhance the performance of MotifNet. MotifNet divided the process of scene graph generation into two steps: an object context encoder and an edge context encoder. The object context encoder was proposed to refine object labels and capture the object context. The edge context encoder was designed to predict the relationship predicates of each object pair. Both the object encoder and the edge encoder consisted of Bi-LSTMs for capturing the global context.

**VCTree**: Tang *et al.* [5] placed the instances of an image into a dynamic tree structure and captured the hierarchical contextual information. Compared with the fixed chain structure and dense graph, the proposed dynamic tree adaptively adjusted the structure and captured hierarchical information according to the content. They integrated supervised learning and reinforcement learning for exploring the dynamic tree structure in the image.

*Corresponding author.

| $M$ | mR@20 | mR@50 | mR@100 |
|---|---|---|---|
| $M = 0$ | 12.4 | 16.0 | 17.5 |
| $M = 5$ | 21.5 | 25.7 | 27.5 |
| $M = 10$ | 24.3 | 29.3 | 31.4 |
| $M = 15$ | 24.5 | 29.4 | 31.7 |
| $M = 20$ | 24.3 | 29.2 | 31.5 |

Table 1. Adjustment of the number of common predicates $M$ in the target domain. When $M = 15$, Transformer (BPL) achieves the best results.

**Transformer**: The Transformer [6] structure based on the self-attention mechanism has been utilized to handle problems in natural language and computer vision. Previous works [1, 3, 2] employed the Transformer structure for the scene graph generation task to explore the relational context in the image. In our experiments, we used the model proposed by Tang *et al.* [3]. For the scene graph generation task, the Transformer also used two stages, *i.e.*, an object encoder and an edge encoder, similar to MotifNet.

Because of the two imbalances mentioned in the paper, *i.e.*, semantic space level imbalance and training sample level imbalance, the prediction results of all these models concentrate on common predicates and ignore informative ones. In view of the two imbalances, we propose the *balance adjustment* method to capture precise and rich information in scene graphs.

## 2. Supplementary Quantitative Results

### 2.1. Study of Common Predicates

We examine how the number of common predicate categories ($M$ mentioned in Section 3.3) in the target domain affects the performance of the method, as shown in Table 1. When $M = 15$, Transformer (BPL) achieves the best re-

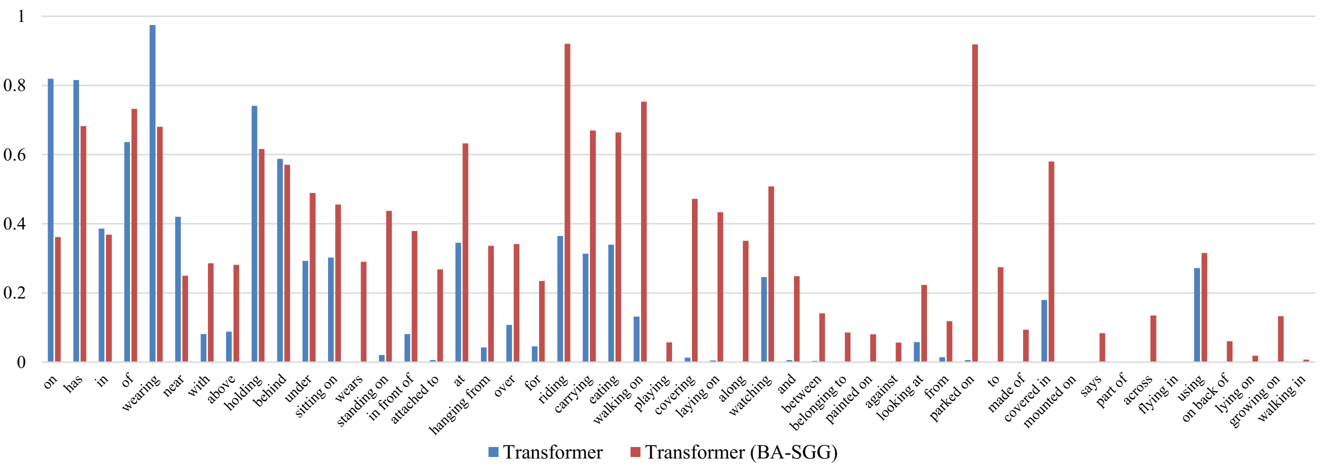


Figure 1. Recall@100 for each predicate on the PredCls task. The performances of Transformer (BA-SGG) are higher than those of Transformer on informative predicates, such as "standing on", "riding" and "parked on".

| $N$ | mR@20 | mR@50 | mR@100 |
|---|---|---|---|
| $N = 2k$ | 24.5 | 29.4 | 31.7 |
| $N = 4k$ | 22.7 | 27.4 | 29.5 |
| $N = 6k$ | 21.7 | 26.1 | 28.1 |
| $N = 8k$ | 20.7 | 25.0 | 27.1 |

Table 2. Adjustment of the number of common predicates $N$ in the target domain.

sults. Too many or too few common predicates are not conducive to the learning process of the model. Then we examine how the number of common predicate examples ($N$ mentioned in Section 3.3) in the target domain affects the method. We increase $N$ from $2k$ to $8k$ in Table 2. We can find that the performance of Transformer (BPL) decreases gradually with the increase of $N$.

## 2.2. Comparison between BA-SGG and TDE

Except for the mean recall rates reported in the paper, our method also stabilizes the recall rate to a certain extent. The recall rates of BA-SGG and TDE [4] are shown in Table 3. Most results of BA-SGG are higher than that of TDE, which indicates the reliability and superiority of our method.

## 2.3. Comparison of Predicate Recall between Transformer and Transformer (BA-SGG)

Figure 1 shows the Recall@100 of each predicate for Transformer and Transformer (BA-SGG) on the PredCls task. Except for a few common predicates, such as "on", "has" and "near", the performances of Transformer (BA-SGG) are better than Transformer for numerous informative predicates, *e.g.*, "standing on", "riding" and "parked on". This shows that the predicate predicted by our method contains more specific information than that of Transformer.

## 3. Supplementary Visualization Results

We show the visualization results of some complex scenes in Figure 2. Our method handles these complex scenes well and generates some informative predicates, such as "walking on", "riding" and "looking at". However, some fine-grained location relationships are still mispredicted, *e.g.*, {shoe, on, bed} in the seventh image and {man, at, table} in the eighth image.

## 4. Conclusion

In this supplementary material, we review the baseline models and show some quantitative and qualitative results. These results illustrate that our method generates reliable scene graphs and adapts to complex scenes well.

## References

[1] Yuyu Guo, Jingkuan Song, Lianli Gao, and Heng Tao Shen. One-shot scene graph generation. In *ACMMM*, 2020.

[2] Rajat Koner, Poulami Sinhamahapatra, and Volker Tresp. Relation transformer network. *CoRR*, abs/2004.06193, 2020.

[3] Kaihua Tang. A scene graph generation codebase in pytorch, 2020. `https://github.com/KaihuaTang/Scene-Graph-Benchmark.pytorch`.

[4] Kaihua Tang, Yulei Niu, Jianqiang Huang, Jiaxin Shi, and Hanwang Zhang. Unbiased scene graph generation from biased training. In *CVPR*, 2020.

[5] Kaihua Tang, Hanwang Zhang, Baoyuan Wu, Wenhan Luo, and Wei Liu. Learning to compose dynamic tree structures for visual contexts. In *CVPR*, 2019.

[6] Ashish Vaswani, Noam Shazeer, Niki Parmar, Jakob Uszkoreit, Llion Jones, Aidan N. Gomez, Lukasz Kaiser, and Illia Polosukhin. Attention is all you need. In *NeurIPS*, 2017.

[7] Rowan Zellers, Mark Yatskar, Sam Thomson, and Yejin Choi. Neural motifs: Scene graph parsing with global context. In *CVPR*, 2018.

| Method | PredCls | | | SGCls | | | SGDet | | |
|---|---|---|---|---|---|---|---|---|---|
| | R@20 | R@50 | R@100 | R@20 | R@50 | R@100 | R@20 | R@50 | R@100 |
| VCTree (TDE) | 36.2 | 47.2 | 51.6 | 19.9 | 25.4 | 27.9 | 14.0 | 19.4 | 23.2 |
| VCTree (BA-SGG) | 43.9 | 50.0 | 51.8 | 30.2 | 34.0 | 35.0 | 15.8 | 21.7 | 25.5 |
| MotifNet (TDE) | 38.7 | 50.8 | 55.8 | 21.8 | 27.2 | 29.5 | 5.9 | 7.4 | 8.4 |
| MotifNet (BA-SGG) | 44.4 | 50.7 | 52.5 | 26.9 | 30.1 | 31.0 | 16.8 | 23.0 | 26.9 |

Table 3. Comparison between BA-SGG and TDE on Recall. Most results of our model (BA-SGG) are better than those of TDE, which illustrates that the scene graphs generated by our method are more reliable than those of TDE.

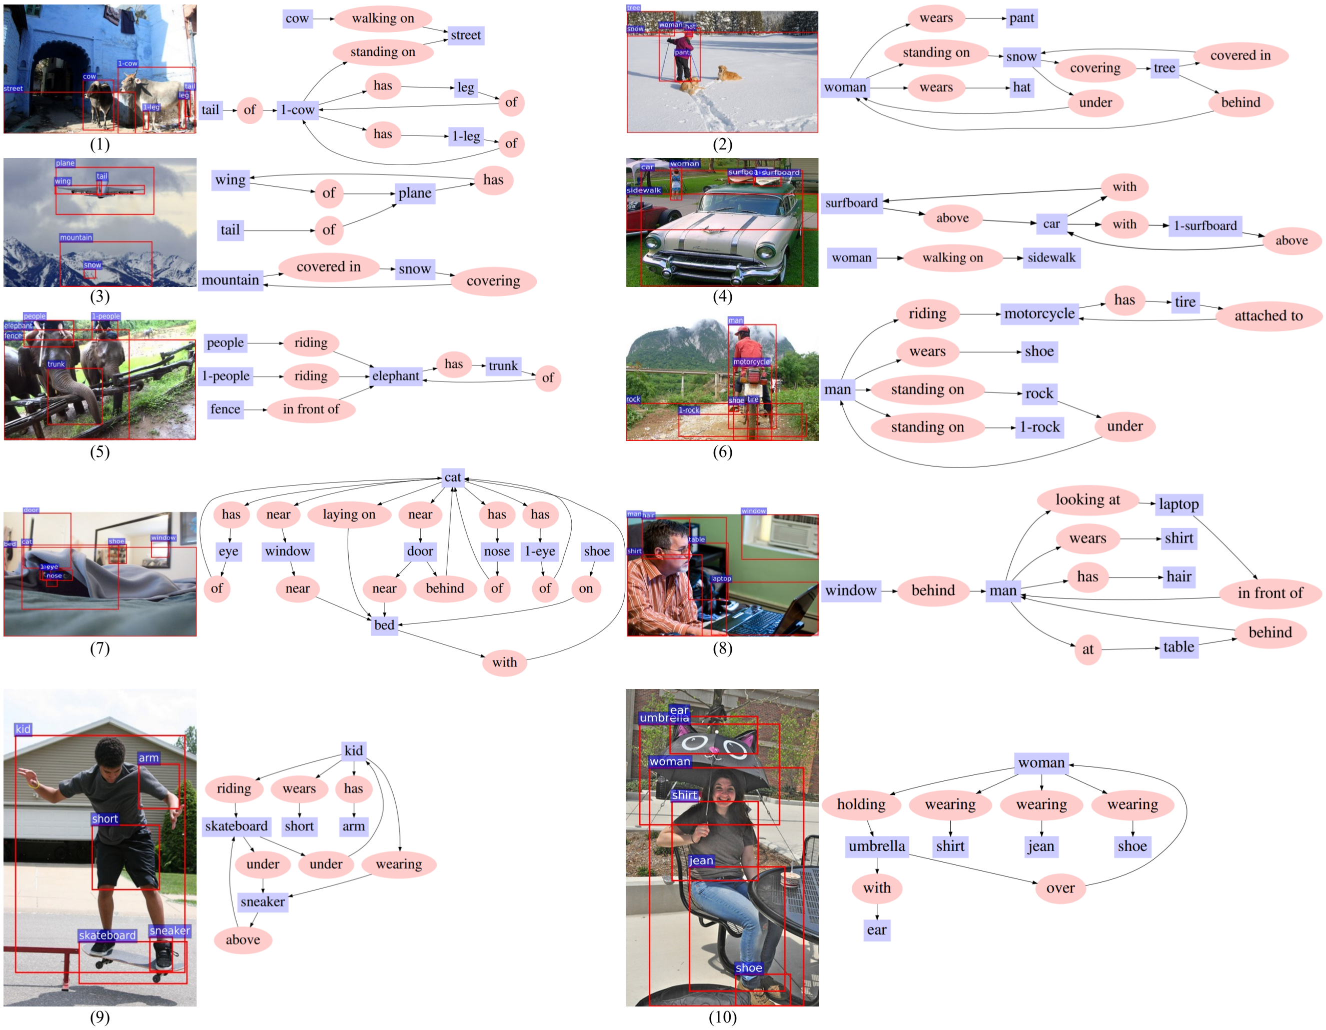


Figure 2. Visualization results of Transformer (BA-SGG) on the PredCls task. Our approach adapts to these complex scenes appropriately and generates some informative predicates, such as "walking on" in the first image, "riding" in the fifth image and "looking at" in the eighth image.
